# Supplementary material for: Large Microwave Inductance of Granular Boron-Doped Diamond Superconducting Films
Source: arXiv:2103.14738 ancillary file (2021-06-16)
Supplement: Supplementary file 1 [file Supplementary_Material.pdf]

## Supplementary Information

Bakhrom Oripov,<sup>1, a)</sup> Dinesh Kumar,<sup>2</sup> Cougar Garcia,<sup>1, 3</sup> Patrick Hemmer,<sup>1</sup> T. Venkatesan,<sup>4, 5</sup> M. S. Ramachandra Rao,<sup>2</sup> and Steven M. Anlage<sup>1, 3</sup>

<sup>1)</sup>*Quantum Materials Center, Physics Department,*

*University of Maryland, College Park, MD 20742, USA*

<sup>2)</sup>*Nano Functional Materials Technology Centre and Materials Science Research Centre, Department of Physics, Indian Institute of Technology (IIT) Madras, Chennai 600036, India*

<sup>3)</sup>*Materials Science and Engineering Department,*

*University of Maryland, College Park, MD 20742, USA*

<sup>4)</sup>*NUSNNI NanoCore, National University of Singapore, 117411, Singapore*

<sup>5)</sup>*Neocera LLC, Beltsville, MD 20705, USA*

(Dated: 26 March 2021)

This is the supplementary information for the "Large Microwave Inductance of Granular Boron-Doped Diamond Superconducting Films" article. The document contains three sections:

### 1. Film Microstructure

In this section, the parameters used in film preparation and corresponding surface microstructure are described in detail.

### 2. Granular Screening Model

In this section, a model of screening in granular superconductors is discussed.

### 3. Surface Resistance

In this section, the surface losses of these Boron-Doped Diamond are estimated and fit.

---

<sup>a)</sup>Electronic mail: bakhromtjk@gmail.com

TABLE I. Summary of the MPCVD deposition conditions and physical properties for all samples.

| Sample | Original label | Substrate | Growth duration | Film thickness $t$ | $\rho(T > T_c)$            | $T_c(\text{Onset})$ | $T_c(\rho = 0)$ |
|--------|----------------|-----------|-----------------|--------------------|----------------------------|---------------------|-----------------|
| A      | D9             | Si(100)   | 3h              | $1.5\mu m$         | $5.5\text{ m}\Omega - cm$  | 7.2K                | 6.4K            |
| B      | TH-7           | Si(100)   | 7h              | $3.5\mu m$         | $9.8\text{ m}\Omega - cm$  | 3.4K                | 2.1K            |
| C      | TH-8           | Si(100)   | 8h              | $4.0\mu m$         | $2.91\text{ m}\Omega - cm$ | 3.5K                | 2.6K            |

## I. FILM MICROSTRUCTURE

Figure 1 shows a plan-view SEM image of sample "A". The surface grain sizes range from less than 100 nm to about 500 nm. Figure 2 shows a cross-sectional SEM image of sample A. The granular nature of the film is also evident here. The film thickness is approximately  $1.5\mu m$ . All the samples were deposited on a diamond-seeded Si substrate. Table I summarizes the deposition conditions and properties of the the films measured in this study.

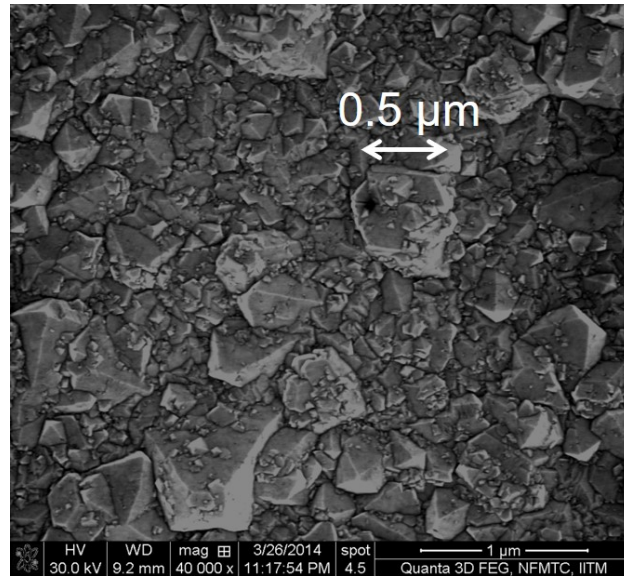

FIG. 1. SEM image of film "A" as measured by a field emission scanning electron microscope (FESEM, Quanta 3D, FEI). The film is highly granular with grain sizes up to  $\sim 0.5\mu m$ .

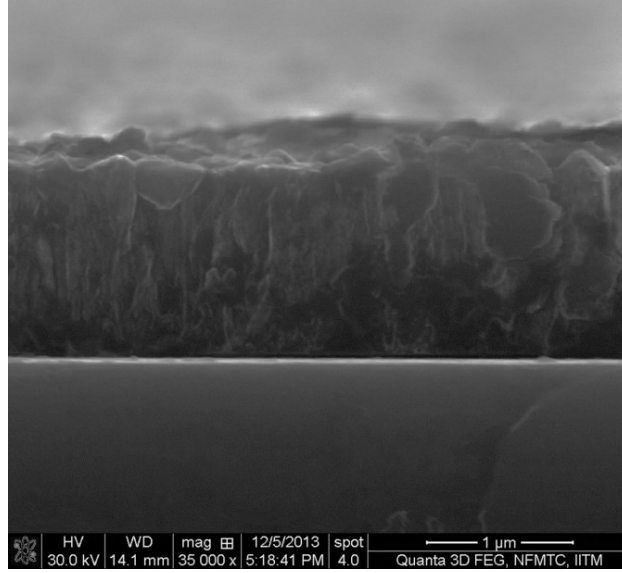

FIG. 2. Field emission scanning electron microscope (FESEM, Quanta 3D, FEI) image of film "A" in cross section, from which the thickness is estimated. The Si substrate is shown at the bottom.

## II. SCREENING LENGTH IN GRANULAR SUPERCONDUCTORS

The objective is to derive expressions for the zero temperature screening length of a granular thin film superconductor. We begin with the laminar model for electromagnetic screening in inhomogeneous superconducting films of thickness  $t$ .<sup>1</sup> This model assumes that grains of characteristic size  $a$  are separated by barriers of thickness  $t_{\text{barrier}}$  periodically in space. The barriers are Josephson contacts that interrupt the current flow, leading to enhanced effective screening length. The Josephson contact is characterized by critical current density  $J_c(T)$ . In the limit of very small grain size and very weak coupling between the grains,<sup>1</sup> the effective screening length becomes  $\lambda_{\text{eff}} = \sqrt{\frac{\Phi_0}{2\pi J_c \mu_0 a}}$ , where  $\Phi_0 = h/2e$  is the superconducting flux quantum. Note that this differs from the expression for the Josephson screening length  $\lambda_J = \sqrt{\frac{\Phi_0}{2\pi J_c \mu_0 d_{\text{eff}}}}$  in the presence of the length scale  $d_{\text{eff}}$  rather than the grain size  $a$ , where  $d_{\text{eff}} = t_{\text{barrier}} + 2\lambda \tanh(t/\lambda)$  is the electromagnetic thickness of the junction, where  $\lambda$  is the screening length in the grains.

We next assume that the critical current is that associated with a single grain boundary, so that  $J_c = I_c/ta$ . Next we assume that the  $I_c R_N$  product of the junction is governed by the Ambegaokar-Baratoff expression<sup>2</sup> at zero temperature,  $I_c(0)R_N(0) = \frac{\pi\Delta(0)}{2e}$ , where  $e$  is the electronic charge. In this case we take  $R_N$  to be the resistance of the barrier material  $R_{\text{barrier}}$ . With these assumptions, the effective screening length of the film becomes  $\lambda_{\text{eff}} = \sqrt{\frac{\hbar t R_{\text{barrier}}}{\pi \mu_0 \Delta(0)}}$ . Writing the resistance of

the barrier in terms of its resistivity and geometrical parameters,  $R_{barrier} = \rho_{barrier} \frac{t_{barrier}}{ta}$ , we have  $\lambda_{eff} = \sqrt{\frac{\hbar \rho_{barrier}}{\pi \mu_0 \Delta(0)}} \sqrt{\frac{t_{barrier}}{a}}$ . Note that the first part of this expression is similar to the conventional expression for a (nominally homogeneous) BCS superconductor in the dirty local limit,  $\lambda_{BCS}^{dirty} = \sqrt{\frac{\hbar \rho_N}{\pi \mu_0 \Delta(0)}}$ , except that the normal state resistivity of the film  $\rho_N$  appears instead of the resistivity of the barrier material. There is an additional factor of  $\sqrt{\frac{t_{barrier}}{a}}$  which is expected to be less than unity. Depending on the resistivity of the barrier material, and its thickness, we expect that  $\lambda_{eff}$  could be greater than, or less than,  $\lambda_{BCS}^{dirty}$ .

### III. SURFACE RESISTANCE

Fig.3 shows the temperature dependence of the effective surface resistance  $R_{eff}(T)$  of the Boron-doped diamond film "A". In this case the Boron doped diamond film "A" was measured using the PPR with a  $d = 75 \mu m$  thick Sapphire dielectric spacer. The entire setup was shielded from ambient magnetic field using a cylindrical Cryoperm magnetic shield.

The effective surface resistance arises from intrinsic BCS contribution and extrinsic contributions<sup>3</sup>

$$R_{eff}(T) = R_{BCS}(T) \times \mathcal{F}(t/\lambda(T)) + R_0, \quad (1)$$

where

$$\frac{R_{BCS}(T)}{R_N} = \sqrt{\frac{\sqrt{(\sigma_1/\sigma_n)^2 + (\sigma_2/\sigma_n)^2} - \sigma_2/\sigma_n}{(\sigma_1/\sigma_n)^2 + (\sigma_2/\sigma_n)^2}},$$

$$\mathcal{F}(t/\lambda(T)) = coth(t/\lambda(T)) + \frac{t/\lambda(T)}{[sinh(t/\lambda(T))]^2}.$$

Here  $R_{BCS}$  is the BCS surface resistance,<sup>4-6</sup> where we numerically solved for  $\frac{\sigma_1(\omega, T)}{\sigma_N}$  and  $\frac{\sigma_2(\omega, T)}{\sigma_N}$  using Mattis-Bardeen theory,<sup>7</sup>  $\mathcal{F}$  is an enhancement factor due to the finite thickness of the film,<sup>3</sup> and  $R_0$  accounts for the assumed temperature independent dielectric loss and radiation loss in the parallel plate resonator.<sup>8-10</sup> Eq.(1) was fit to the surface resistance data (red line in Fig.3) for fixed values of  $\lambda(0) = 4.03 \mu m$ ,  $T_c = 5.69 K$ ,  $\Delta(0) = 1.764 k_B T_c$  which were extracted from the Eq.(1) of the main text fit to the associated  $f_0(T)$  data near 5.3 GHz. The normal state surface resistance of the Boron-doped diamond  $R_N$  and residual loss  $R_0$  were used as the fitting parameters. The most accurate fit to the data was achieved with  $R_N = 853.85 \pm 43.97 m\Omega$ , and  $R_0 = 1.37 \pm 0.02 m\Omega$ . We note that the normal state surface resistance is related to the normal state resistivity as  $R_N = \sqrt{\mu_0 \omega \rho_N / 2}$ . The resulting estimate of  $\rho_N = 3.7 m\Omega - cm$  is close to the independently measured

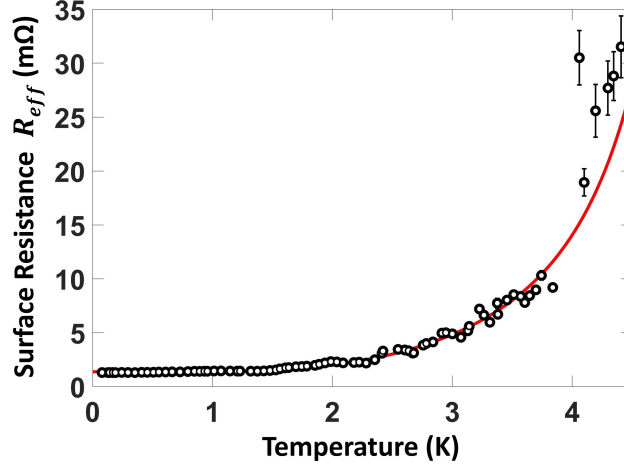

FIG. 3. Effective surface resistance  $R_{eff}$  of the Boron-doped diamond film "A" measured at a frequency of  $f = 4.9 - 5.3$  GHz (black  $\circ$ ). Also shown is the fit to the data (red line) using Eq.(1) with  $\lambda(0) = 4.03 \mu m$ ,  $T_c = 5.69 K$  and  $\Delta(0) = 1.764k_B T_c$  as fixed parameters; and  $R_N = 853.85 \pm 43.97 m\Omega$ ,  $R_0 = 1.37 \pm 0.02 m\Omega$  as fitting parameters.

value of  $\rho_{N,DC} = 5.5 m\Omega - cm$ , giving confidence in this fit. The residual loss  $R_0$  is consistent with the expected extrinsic contributions from radiation loss out the sides of the PPR and through the films, as well as dielectric loss.

## REFERENCES

- <sup>1</sup>T. L. Hylton and M. R. Beasley, "Effect of grain boundaries on magnetic field penetration in polycrystalline superconductors," *Physical Review B* **39**, 9042–9048 (1989).
- <sup>2</sup>V. Ambegaokar and A. Baratoff, "Tunneling between superconductors," *Physical Review Letters* **10**, 486–489 (1963).
- <sup>3</sup>N. Klein, H. Chaloupka, G. Müller, S. Orbach, H. Piel, B. Roas, L. Schultz, U. Klein, and M. Peiniger, "The effective microwave surface impedance of high  $T_c$  thin films," *Journal of Applied Physics* **67**, 6940–6945 (1990).
- <sup>4</sup>J. P. Turneare, J. Halbritter, and H. A. Schwetman, "The surface impedance of superconductors and normal conductors: The Mattis-Bardeen theory," *Journal of Superconductivity* **4**, 341–355 (1991).
- <sup>5</sup>J. Zmuidzinas, "Superconducting Microresonators: Physics and Applications," *Annual Review of Condensed Matter Physics* **3**, 169–214 (2012).

- <sup>6</sup>A. Gurevich, “Theory of RF superconductivity for resonant cavities,” *Superconductor Science and Technology* **30**, 034004 (2017).
- <sup>7</sup>D. C. Mattis and J. Bardeen, “Theory of the Anomalous Skin Effect in Normal and Superconducting Metals,” *Phys. Rev.* **111**, 412–417 (1958).
- <sup>8</sup>R. C. Taber, “A parallel plate resonator technique for microwave loss measurements on superconductors,” *Review of Scientific Instruments* **61**, 2200–2206 (1990).
- <sup>9</sup>M. S. Pambianchi, S. M. Anlage, E. S. Hellman, E. H. Hartford, M. Bruns, and S. Y. Lee, “Penetration depth, microwave surface resistance, and gap ratio in NbN and  $\text{Ba}_{1-x}\text{K}_x\text{BiO}_3$  thin films,” *Applied Physics Letters* **64**, 244–246 (1994).
- <sup>10</sup>V. V. Talanov, L. V. Mercaldo, S. M. Anlage, and J. H. Claassen, “Measurement of the absolute penetration depth and surface resistance of superconductors and normal metals with the variable spacing parallel plate resonator,” *Review of Scientific Instruments* **71**, 2136–2146 (2000).
